# Supplementary material for: Code-Aware Prompting: A study of Coverage Guided Test Generation in Regression Setting using LLM
Source: arXiv:2402.00097 source file (2024-04-02)
Supplement: Supplementary file 1 [file 10_appendix.tex]

\clearpage{}
\appendix

\section{Path Collection Algorithm}
\label{app:path_collection}

\begin{algorithm}
\caption{\label{alg:sympath_generation}Path Constraint Collection}
\footnotesize
\begin{algorithmic}[1]
\Procedure{collectPathConstraints}{focalmethod}
\State root = Parse(focalmethod)
\State active\_paths, terminal\_paths = visitASTNode(root, \{\}, \{\})
\State terminal\_paths = terminal\_paths $\cap$ addReturnValue(active\_paths, \ttt{None})
\State \Comment{Associates a return value \ttt{None} with each path}
\State \Return terminal\_paths
\EndProcedure
% \State
% \Procedure{addReturnValue}{active\_paths, return\_value}
% \State terminal\_paths = \{\}
% \For{path in active\_paths}
%     \State terminal\_paths $\cap =$ (path, return\_value)
% \EndFor
% \State \Return terminal\_paths
% \EndProcedure
% \State
% \Procedure{addConstraint}{active\_paths, constraint}
% \For{path in active\_paths}
%     \State path = path $\land$ constraint
% \EndFor
% \State \Return active\_paths
% \EndProcedure
\State
\Procedure{visitASTNode}{node, active\_paths, terminal\_paths}
\If{node is an if statement}
    \State if\_constraint = extractConstraint(node)
    \State if\_block = getChildBlock(node)
    \State if\_paths = addConstraint(active\_paths, if\_constraint)
    \State active\_paths, terminal\_paths = visitASTNode(if\_block, if\_paths, terminal\_paths)
    \State inv\_constraints = $\neg$if\_constraint)
    \For{child in getChildren(node)}
        \If{child is an elif statement}
            \State elif\_block = getChildBlock(node)
            \State elif\_constraint = extractConstraint(node)
            \State elif\_paths = addConstraint(active\_paths, inv\_constraints $\land \neg$ elif\_constraint)
            \State active\_paths, terminal\_paths = visitASTNode(elif\_block, elif\_paths)
            \State inv\_constraints = inv\_constraints $\cap$ invert(elif\_constraint)
        \ElsIf{child is an else statement}
            \State else\_block = getChildBlock(node)
            \State else\_paths = addConstraint(active\_paths, inv\_constraints)
            \State active\_paths, terminal\_paths = visitASTNode(else\_block, else\_paths)
        \EndIf
    \EndFor
    \If{if node does not have an \ttt{else} child clause}
        \State else\_paths = add\_constraint(active\_paths, inv\_constraints)
        \State active\_paths = active\_paths $\cup$ else\_paths
    \EndIf
\ElsIf{node is a while statement}
    \State while\_constraint = extractConstraint(node)
    \State while\_block = getChildBlock(node)
    \State while\_paths = addConstraint(active\_paths, if\_constraint)
    \State active\_paths, terminal\_paths = visitASTNode(while\_block, if\_paths, terminal\_paths)
    \State not\_while\_paths = addConstraint(active\_paths, $\neg$ while\_constraint)
    \State active\_paths = active\_paths $\cup$ not\_while\_paths
\ElsIf{node is a return statement}
    \State return\_value = extractValue(node)
    \State terminal\_paths = terminal\_paths $\cap$ addReturnValue(active\_paths, return\_value)
    \State active\_paths = \{\}
\Else
    \For{child in getChildren(node)}
        \State active\_paths, terminal\_paths = visitASTNode(child, active\_paths, terminal\_paths)
    \EndFor
\EndIf
\State active\_paths = linearizePaths(active\_paths)
\State \Return active\_paths, terminal\_paths
\EndProcedure
\end{algorithmic}
\end{algorithm}

The detailed algorithm is shown in Algorithm \ref{alg:sympath_generation}. 
\tsc{collectPathConstraints} first parses the relevant focal method and then calls \tsc{visitASTNode} on the root of the focal method AST. \tsc{visitASTNode} maintains two lists: \ttt{active\_paths} is a list of possible execution path constraints that must be satisfied to reach the current node in the AST, and \ttt{terminal\_paths}, a list of execution path constraints that terminate at previously visited \ttt{return} statements. Each terminal path is associated with the return value of the return statement where it terminates and represented internally as a $(\ttt{path\_constraint}, \ttt{return\_expr})$ tuple.

The procedure \tsc{visitASTNode} performs a preorder traversal of the focal method AST.
When \tsc{visitASTNode} visits an AST node, it can do one of three things: if the node is an \ttt{if} or \ttt{loop} statement, the visitor will collect relevant constraints and visits the child code blocks of the conditional AST node.
% ~\bray{what happens to for loop?} 
When traversing branch conditions and loops, the analysis adds additional paths to active path set to cover cases where the branch or loop constraint is satisfied or inverted. When branches have multiple exclusive constraints \eg{\ttt{else-if} or \ttt{else}}, the previous branch conditions are included as inverted constraints. 
If the node is a return statement, the visitor will convert all active paths to terminal paths based on the return statement expression. If the the node is neither a conditional statement or return statement, the visitor traverses each of the node children in order.

When the visitor reaches an \ttt{if} statement, it extracts the \ttt{if} condition and visits the \ttt{if} statement's child block with an updated list of active paths that include the if condition. This models the constraints that need to be met in order for any execution to cover the code block under the if statement. After visiting the \ttt{if} child block, the visitor visits each of the \ttt{elif} and \ttt{else} clauses of the \ttt{if} statement while maintaining a negated set of branch constraints from the previously visited clauses in the branch statement. Each \ttt{elif} clause then uses the negated constraints of the previous \ttt{if} and \ttt{elif} that it uses to construct the specific path constraint associated with its child block, while the \ttt{else} clause uses the negated conditions of the \ttt{if} and all \ttt{elif} statements as its path constraint. If the \ttt{if} statement does not have an \ttt{else} clause, a additional path with the negated branch conditions is added to set of active paths to represent the case where the \ttt{if} statement is not executed.

\ttt{While} statements are treated like \ttt{if} statements, where paths for both the \ttt{while} statement executing at least once, and the \ttt{while} not executing and being skipped, are both added to set of active paths. 
When a \ttt{return} statement is reached, all the active execution paths that reach that return statement are converted into terminal paths with the return statement expression, indicating that these of sets of path constraints that will cause focal method to return the expression in the return statement.

\section{Additional Case Studies}
\label{app:case_studies}

\begin{figure}
\centering
    \begin{subfigure}[b]{0.612\linewidth}
    % \begin{subfigure}[b]{0.412\linewidth}
    \centering
        \includegraphics[width=\textwidth]{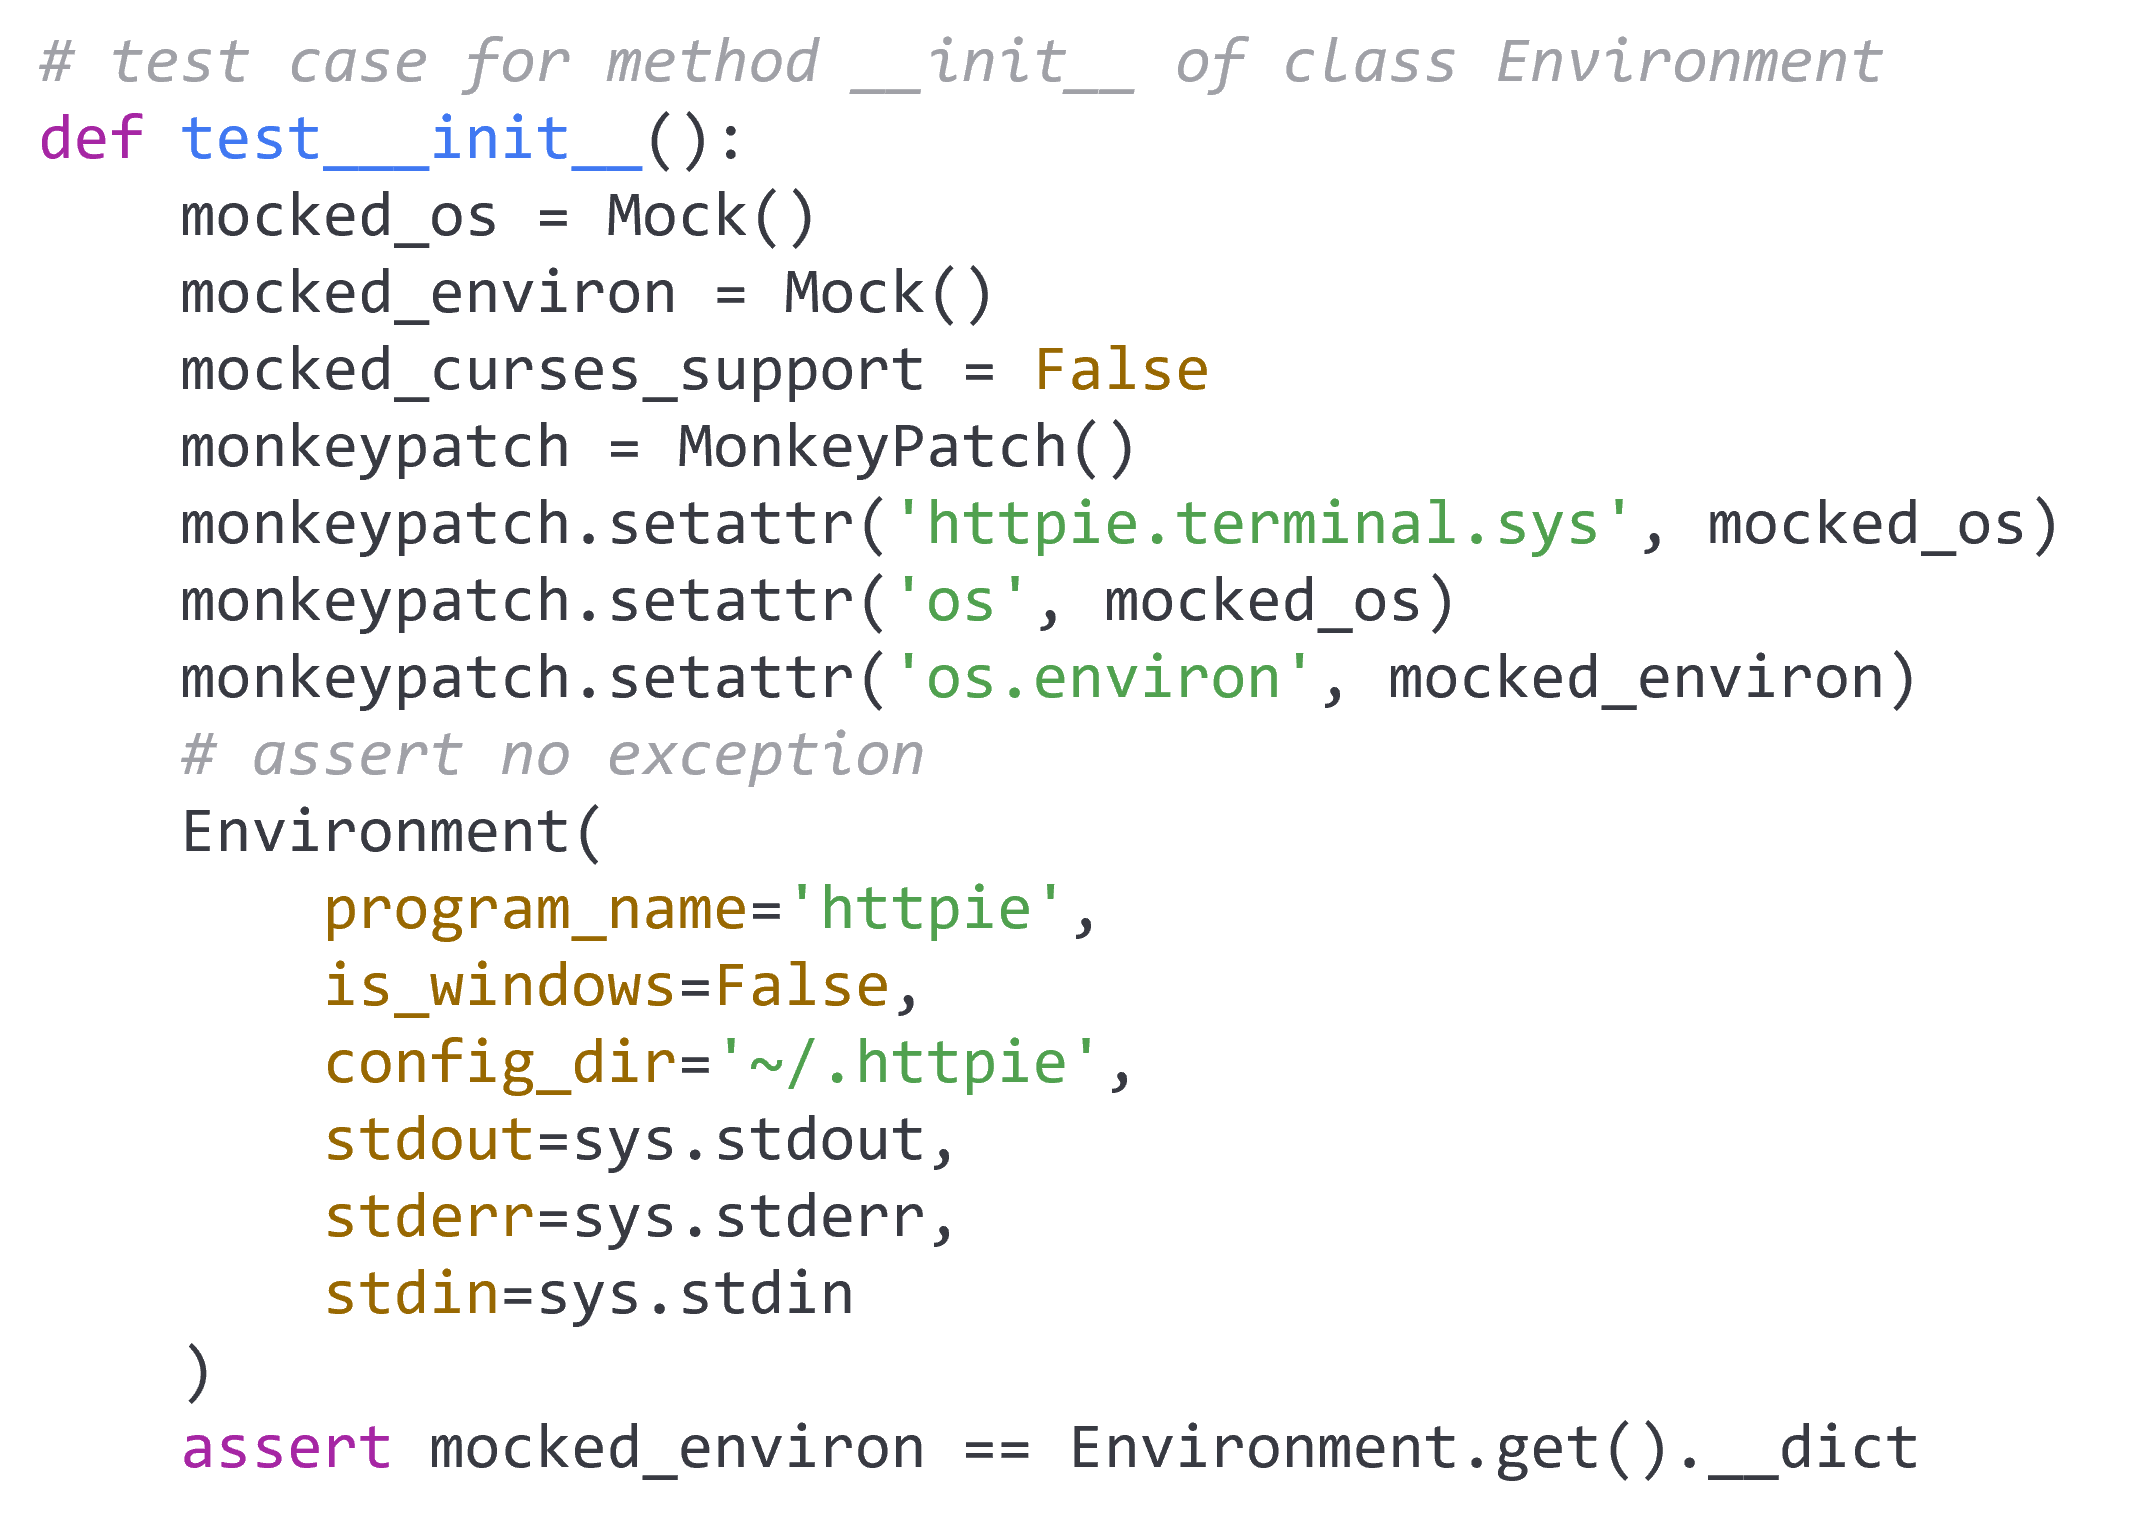}
        % \vspace{-10pt}
        \caption{Baseline test generation.\label{fig:casetudy3:baseline}}
    \end{subfigure}
  \begin{subfigure}[b]{0.86\linewidth}
  % \begin{subfigure}[b]{0.56\linewidth}
  \centering
        \includegraphics[width=\textwidth]{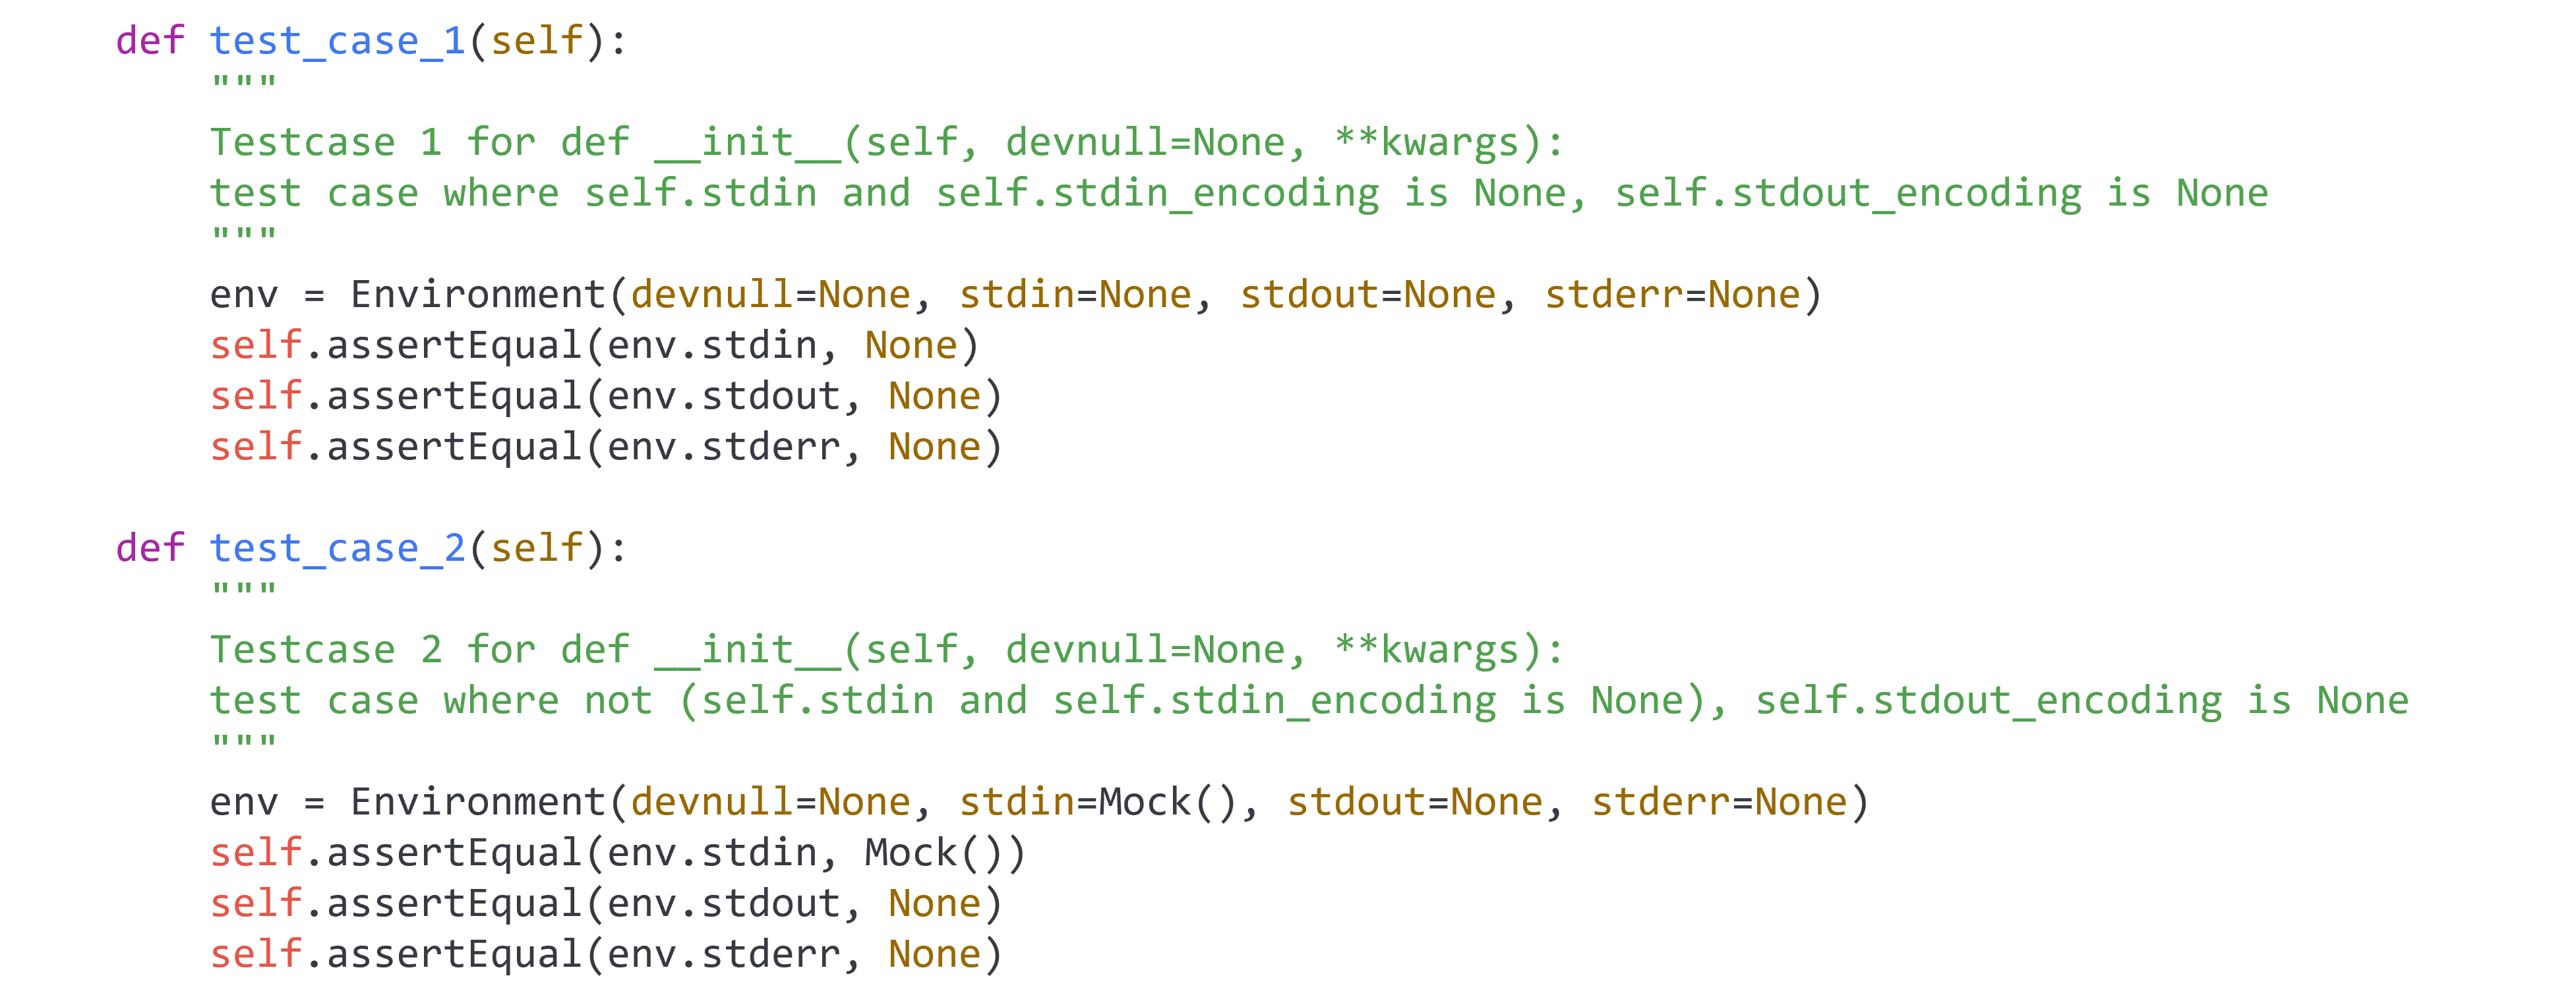}
        % \vspace{-10pt}
        \caption{\approach test generation.\label{fig:casestudy3:symprompt}}
    \end{subfigure}
\caption{Case study where baseline test generation only tests one path and has a misuse error. \approach tests both paths and uses method correctly. Note that in this case the method does not return a value, therefore \approach does not prompt for assertions on the return statement.\label{fig:baselines}}
\end{figure}

\begin{figure}
\centering
    \begin{subfigure}[b]{0.812\linewidth}
    % \begin{subfigure}[b]{0.412\linewidth}
    \centering
        \includegraphics[width=\textwidth]{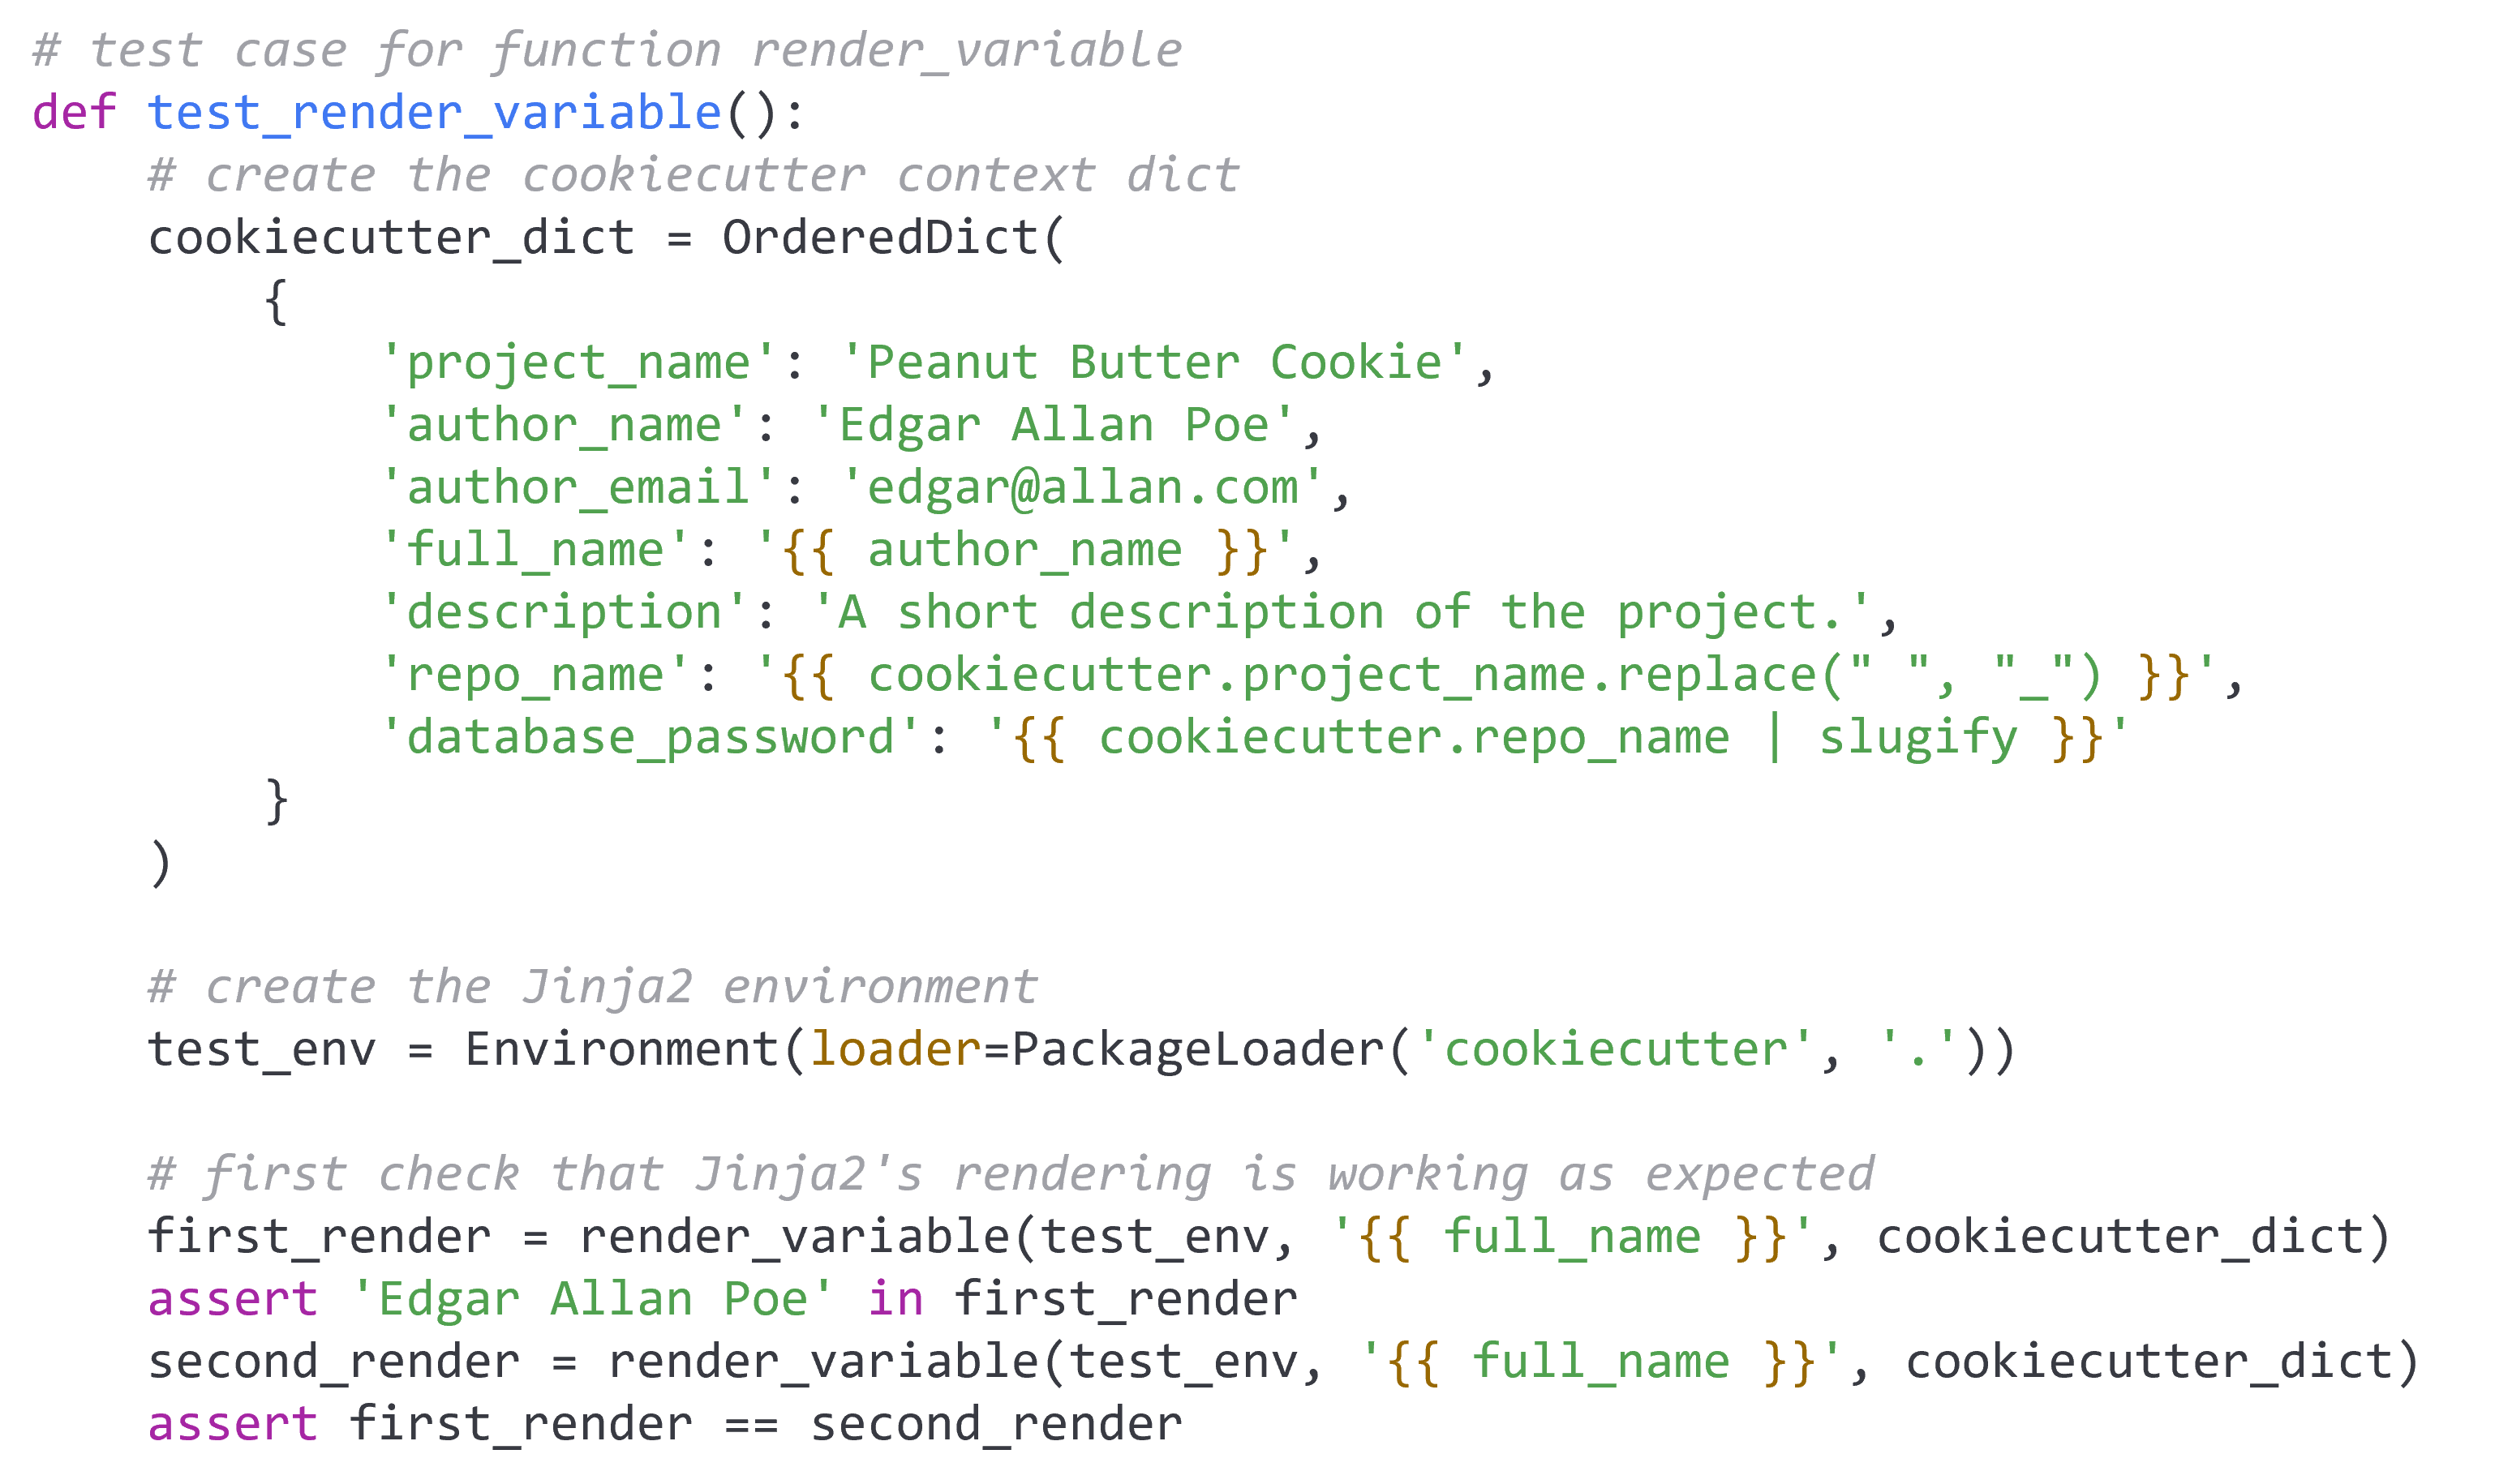}
        % \vspace{-10pt}
        \caption{Baseline test generation.\label{fig:casetudy4:baseline}}
    \end{subfigure}
  \begin{subfigure}[b]{0.86\linewidth}
  % \begin{subfigure}[b]{0.56\linewidth}
  \centering
        \includegraphics[width=\textwidth]{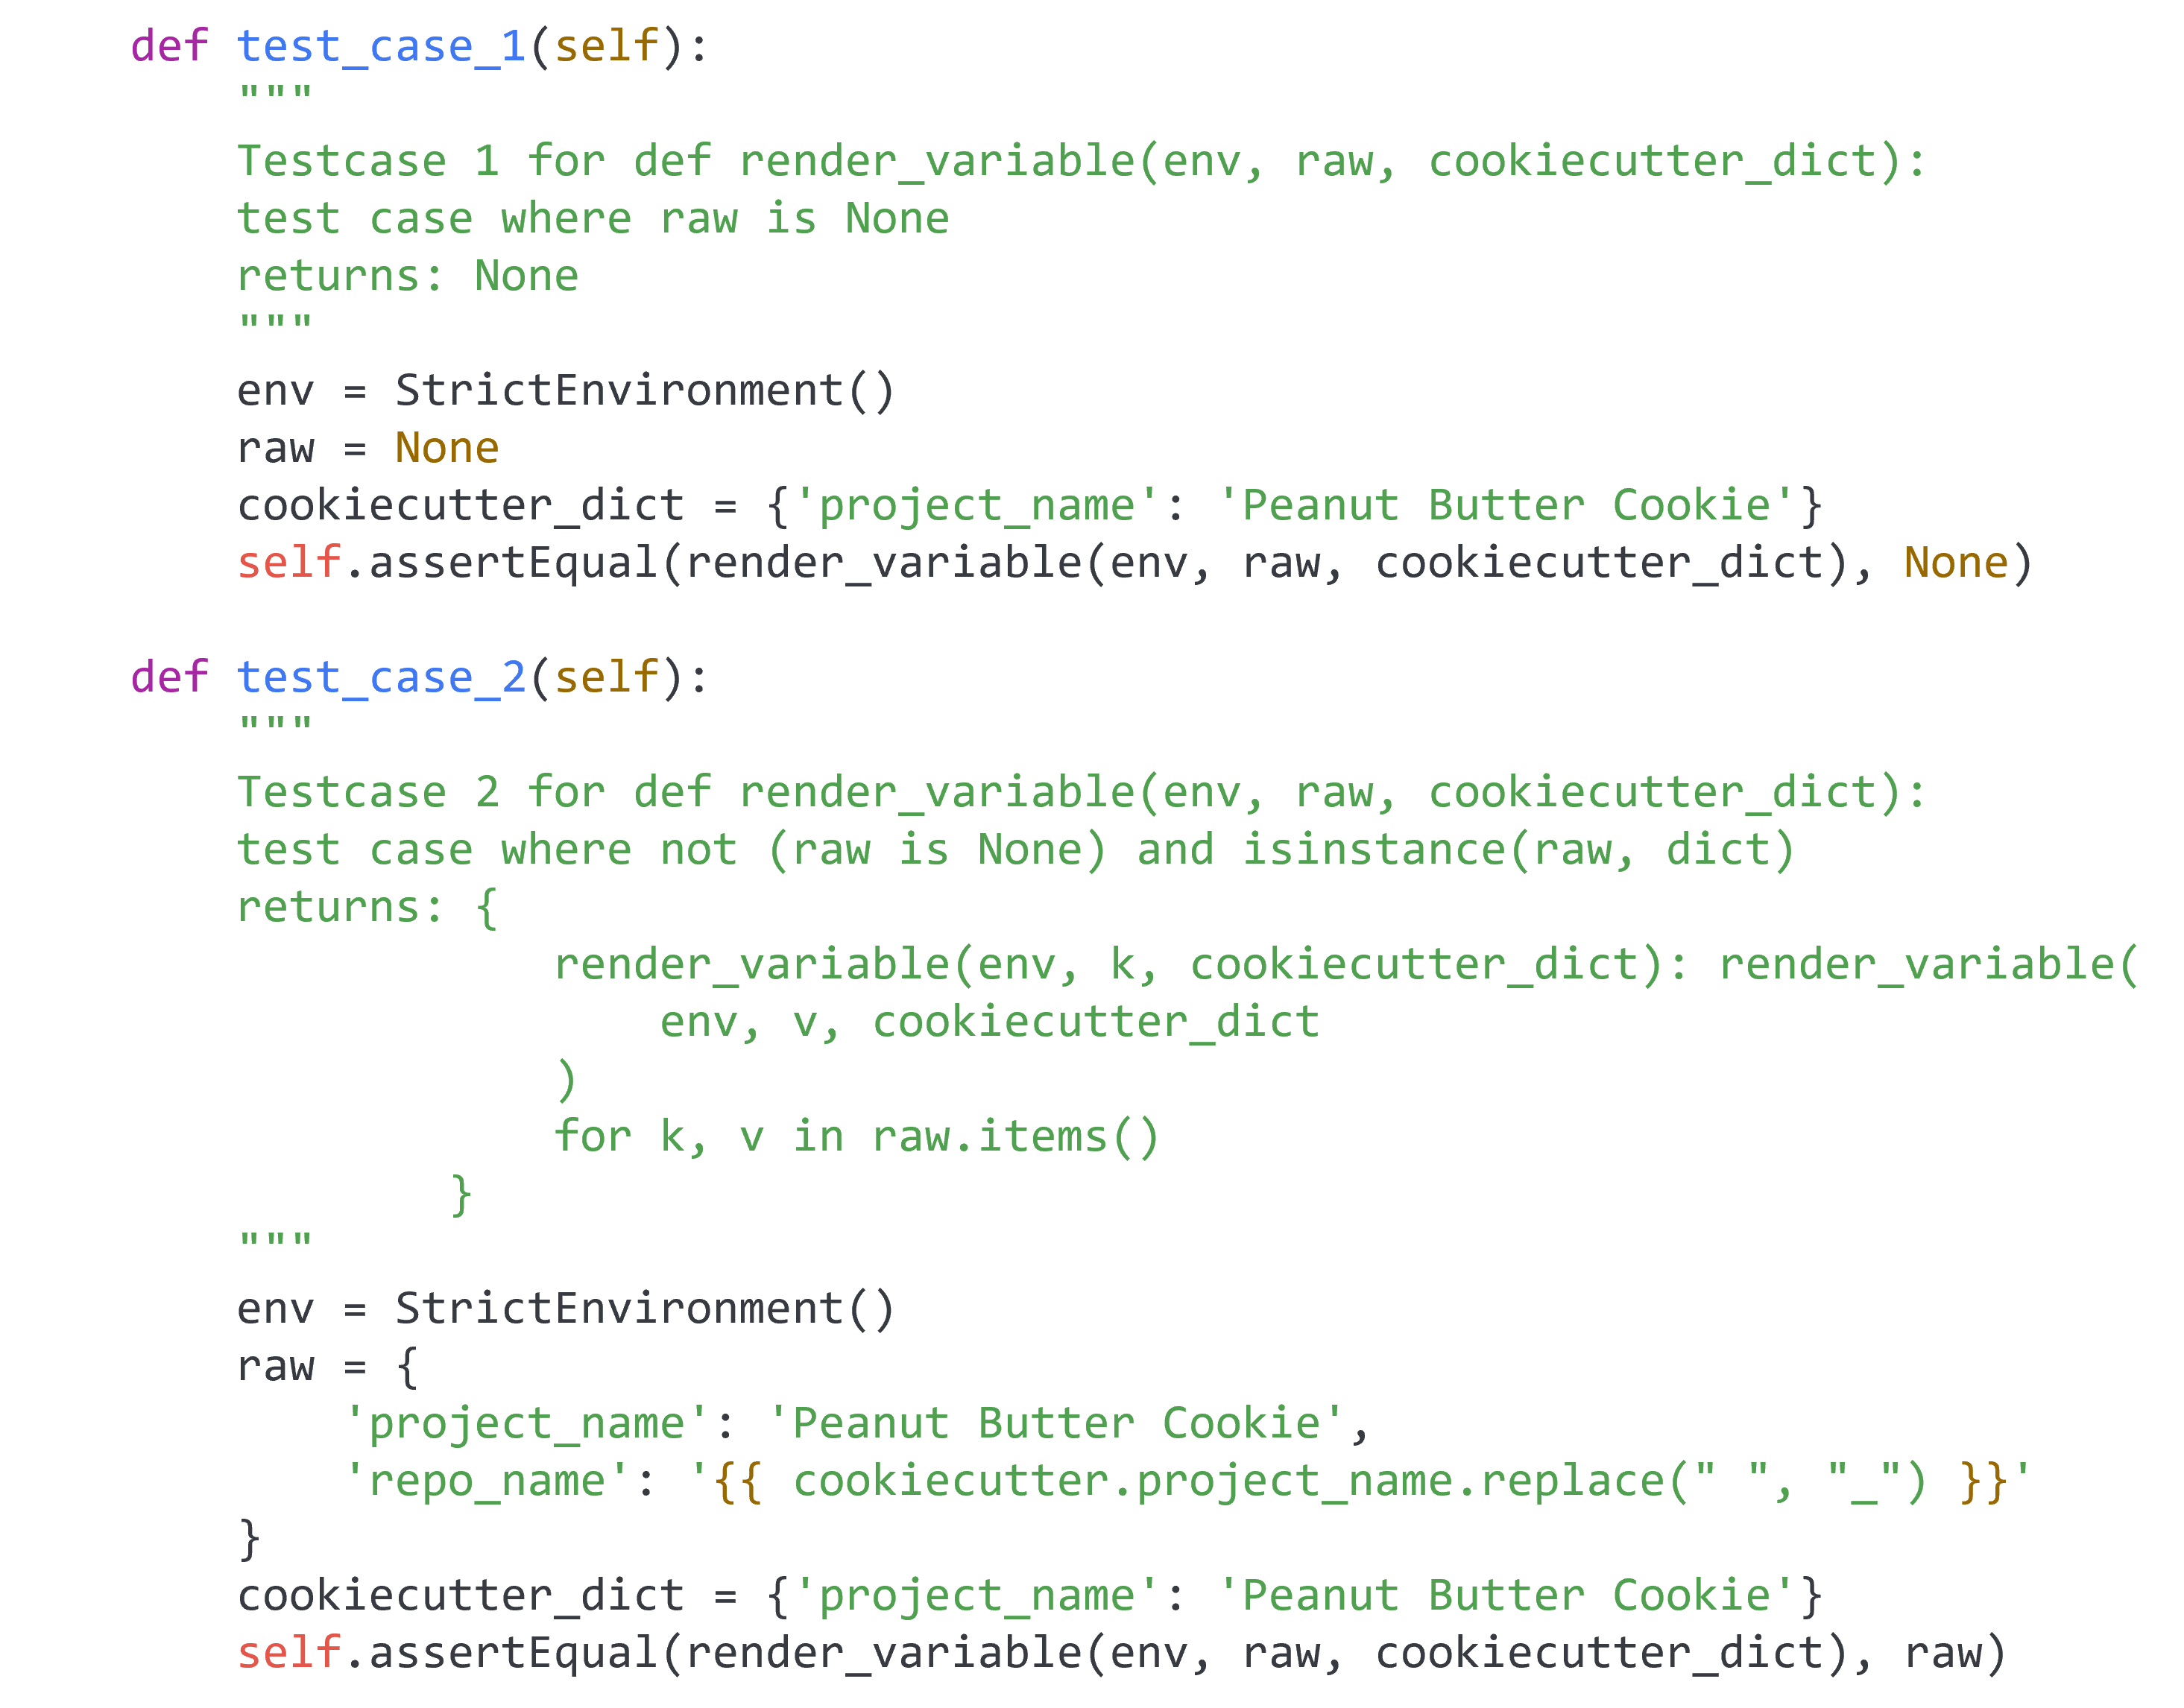}
        % \vspace{-10pt}
        \caption{\approach test generation.\label{fig:casestudy4:symprompt}}
    \end{subfigure}
\caption{Case study where baseline test generation only tests one path and has a misuse error. \approach tests both paths and uses method correctly. Note that in this case the method does not return a value, therefore \approach does not prompt for assertions on the return statement.\label{fig:baselines}}
\end{figure}

\begin{figure}
\centering
    \begin{subfigure}[b]{0.812\linewidth}
    \centering
        \includegraphics[width=\textwidth]{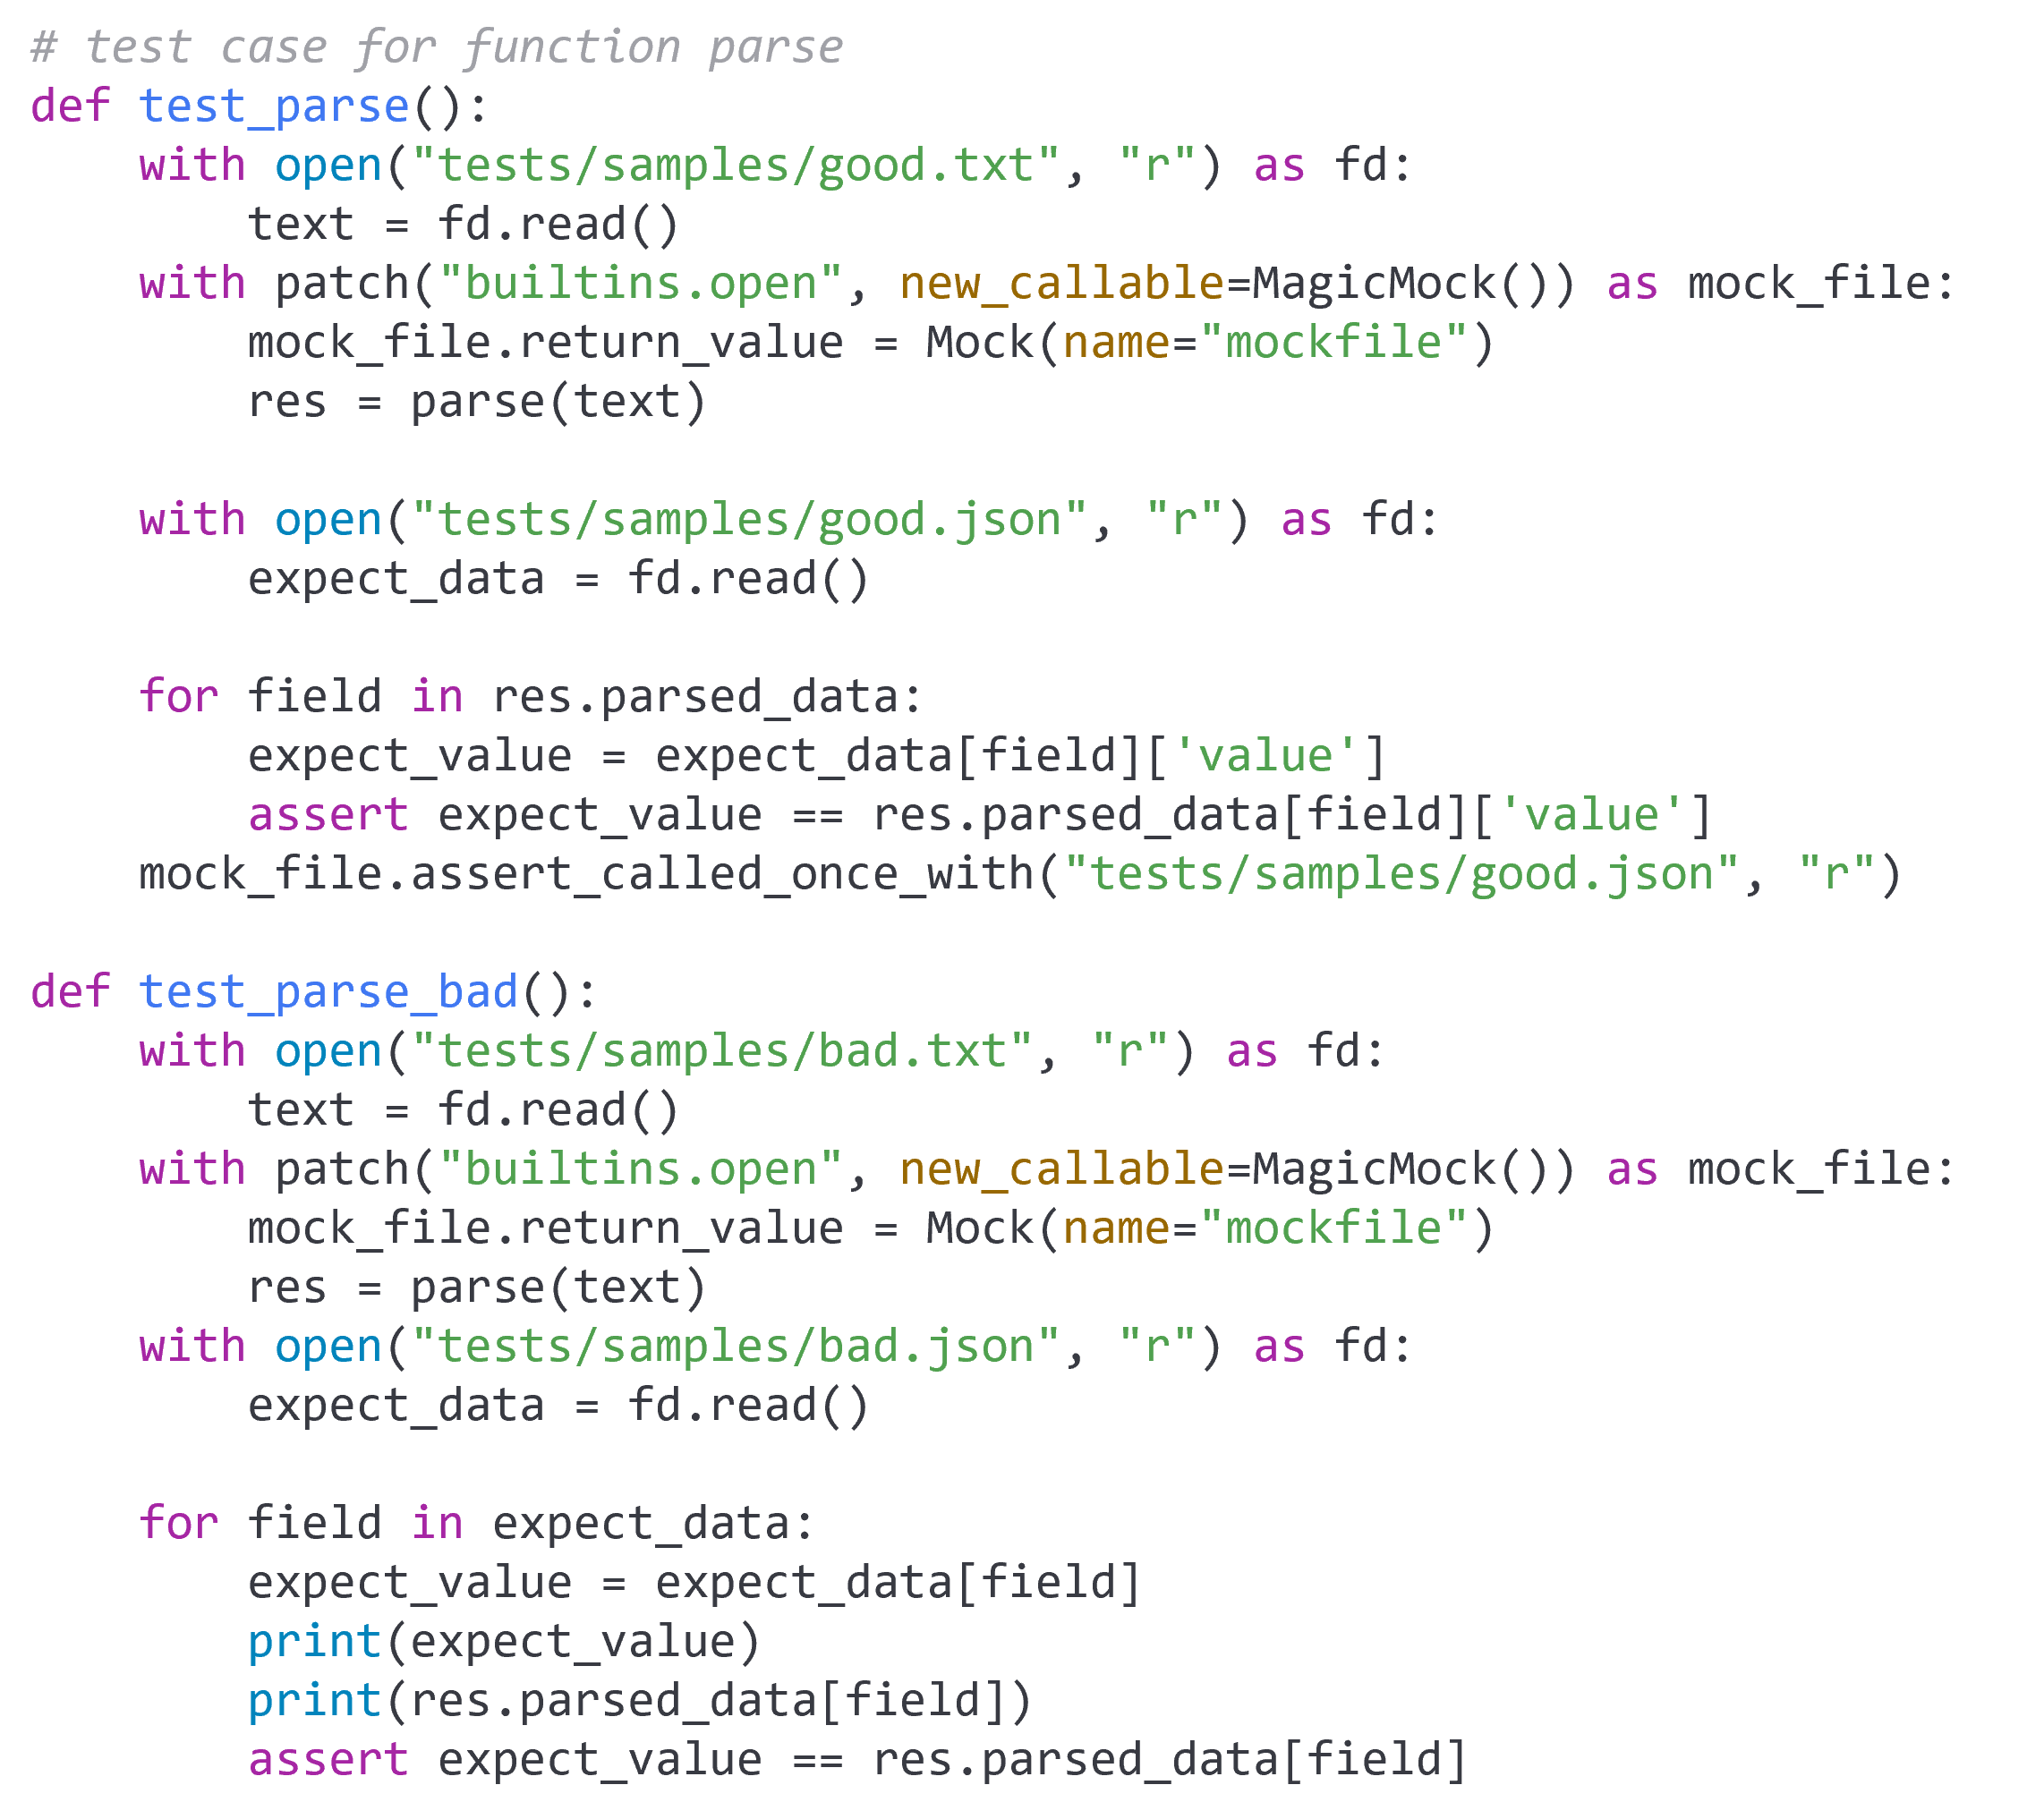}
        % \vspace{-10pt}
        \caption{Baseline test generation.\label{fig:casetudy5:baseline}}
    \end{subfigure}
  \begin{subfigure}[b]{0.86\linewidth}
  \centering
        \includegraphics[width=\textwidth]{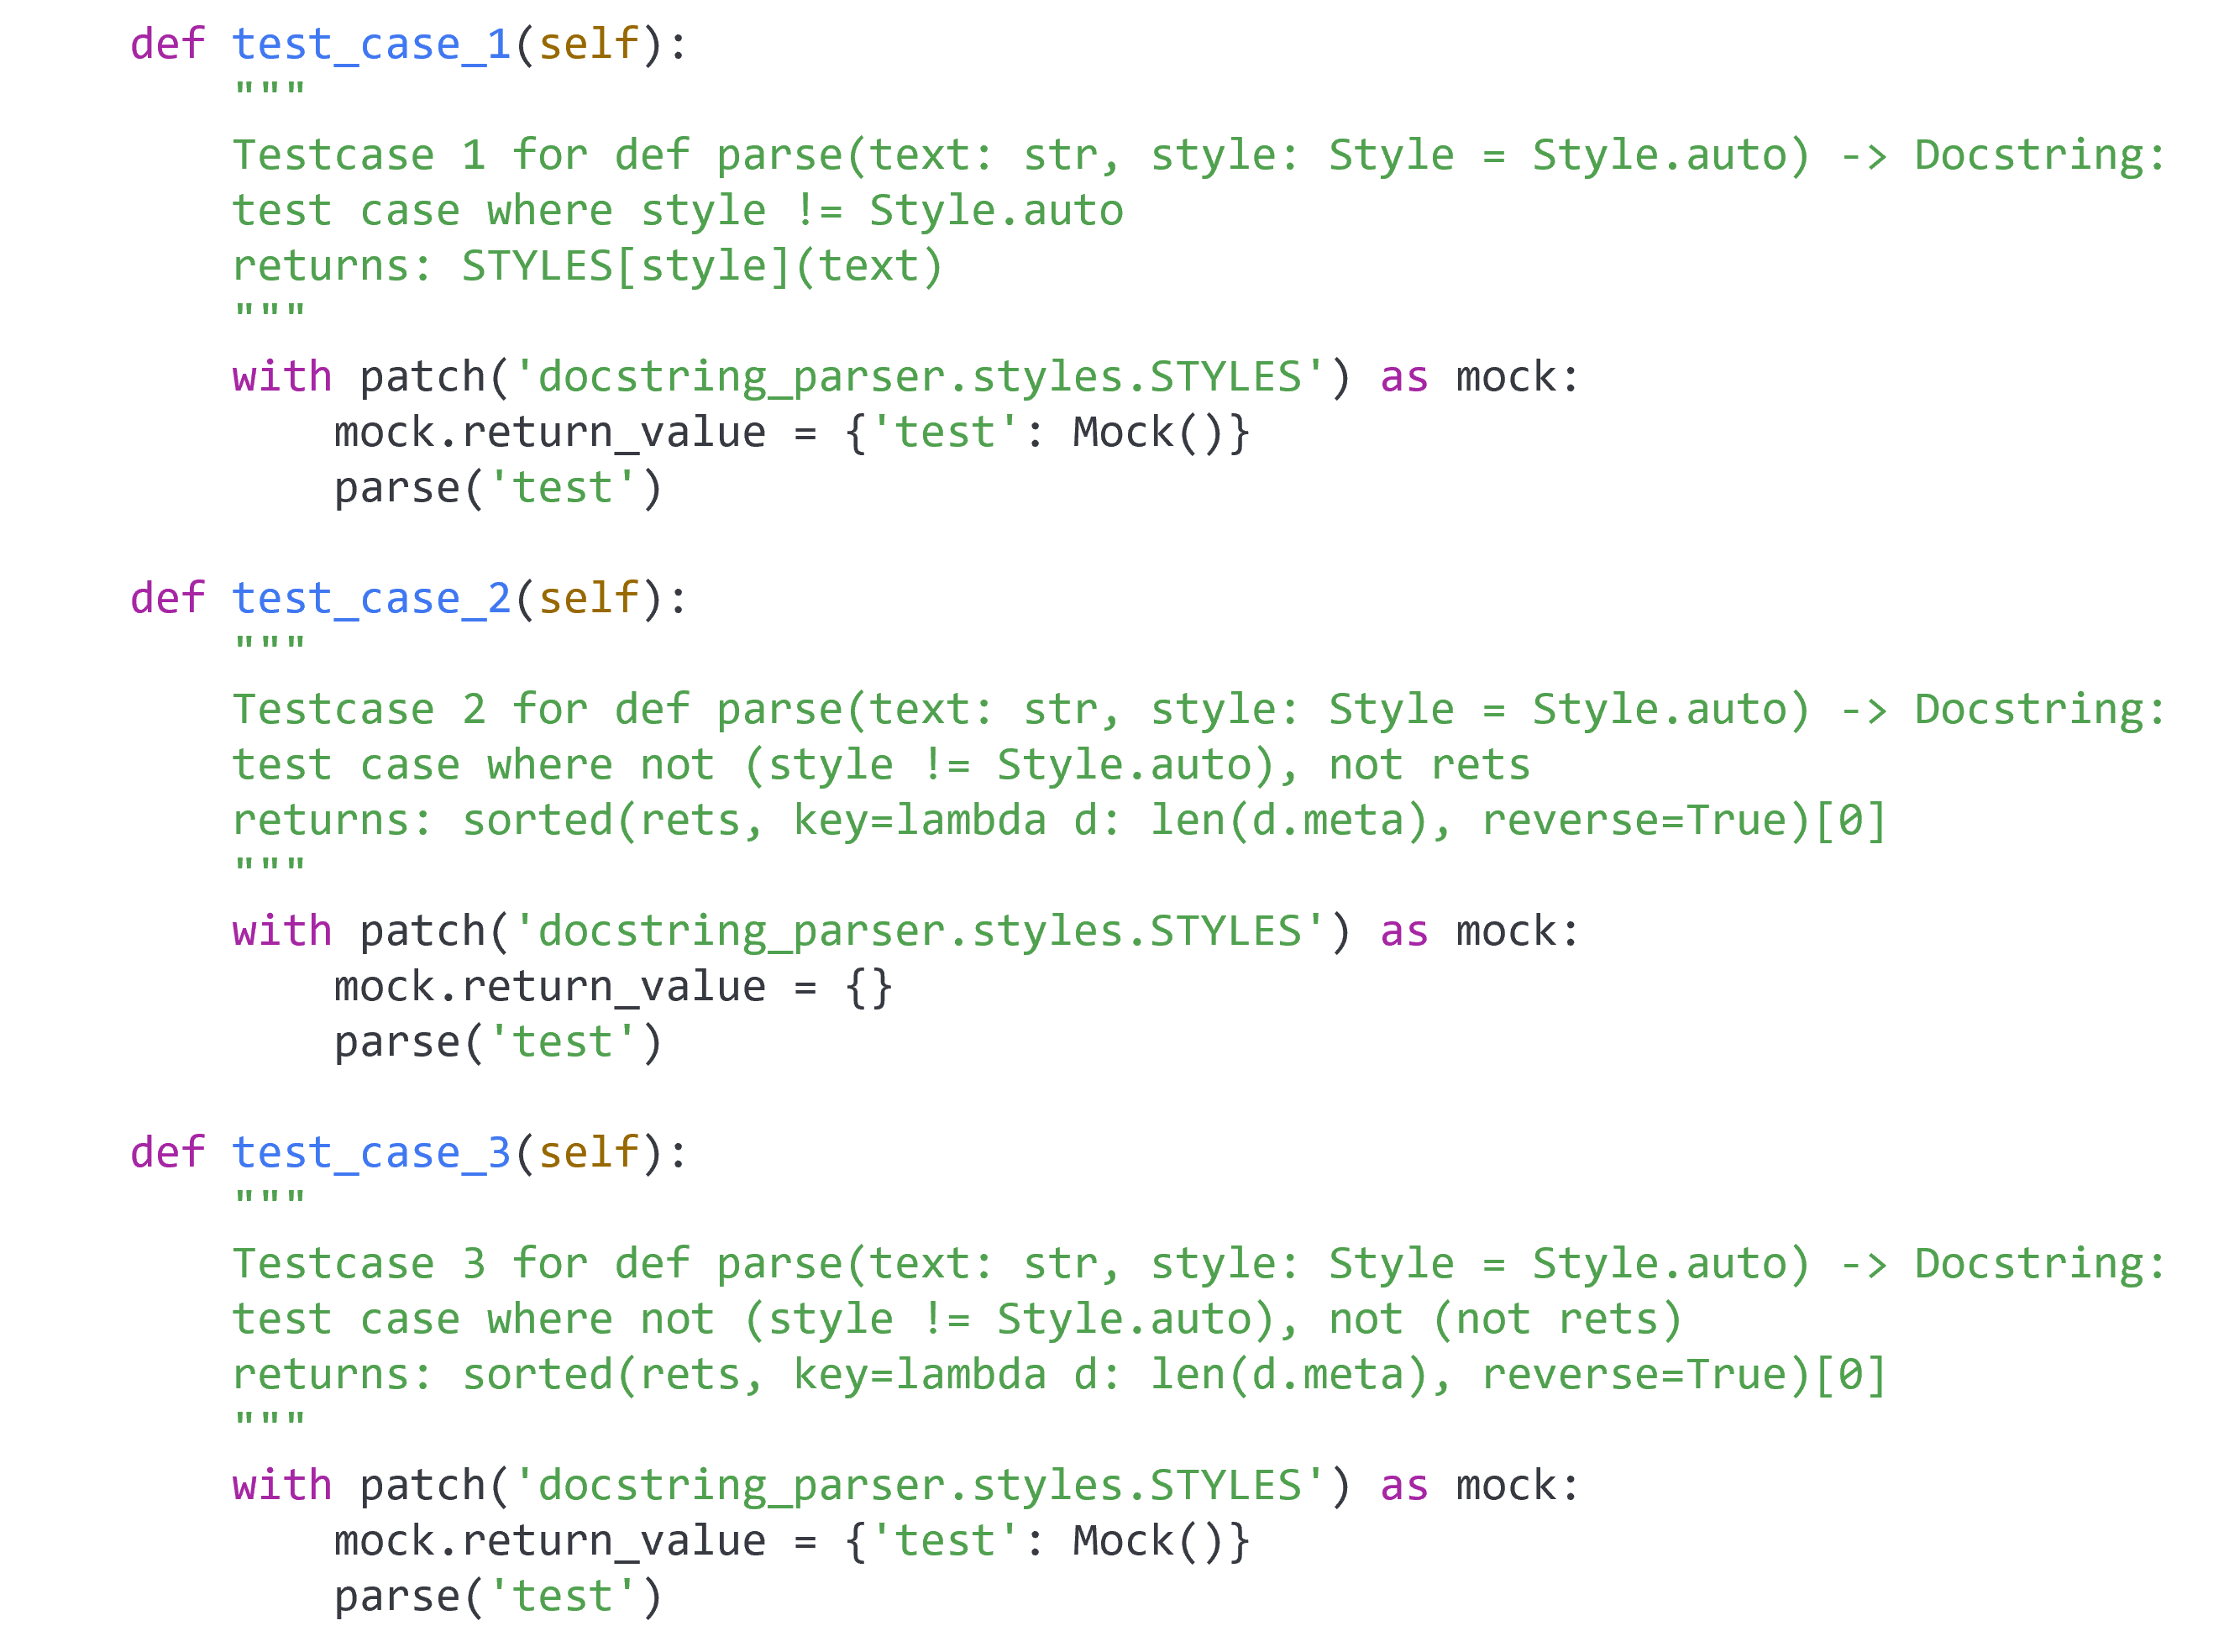}
        % \vspace{-10pt}
        \caption{\approach test generation.\label{fig:casestudy5:symprompt}}
    \end{subfigure}
\caption{Case study where baseline test generation has a misuse error. \approach tests more paths and uses the method correctly. \label{fig:baselines}}
\end{figure}

\begin{figure}
\centering
    \begin{subfigure}[b]{0.8\linewidth}
    \centering
        \includegraphics[width=\textwidth]{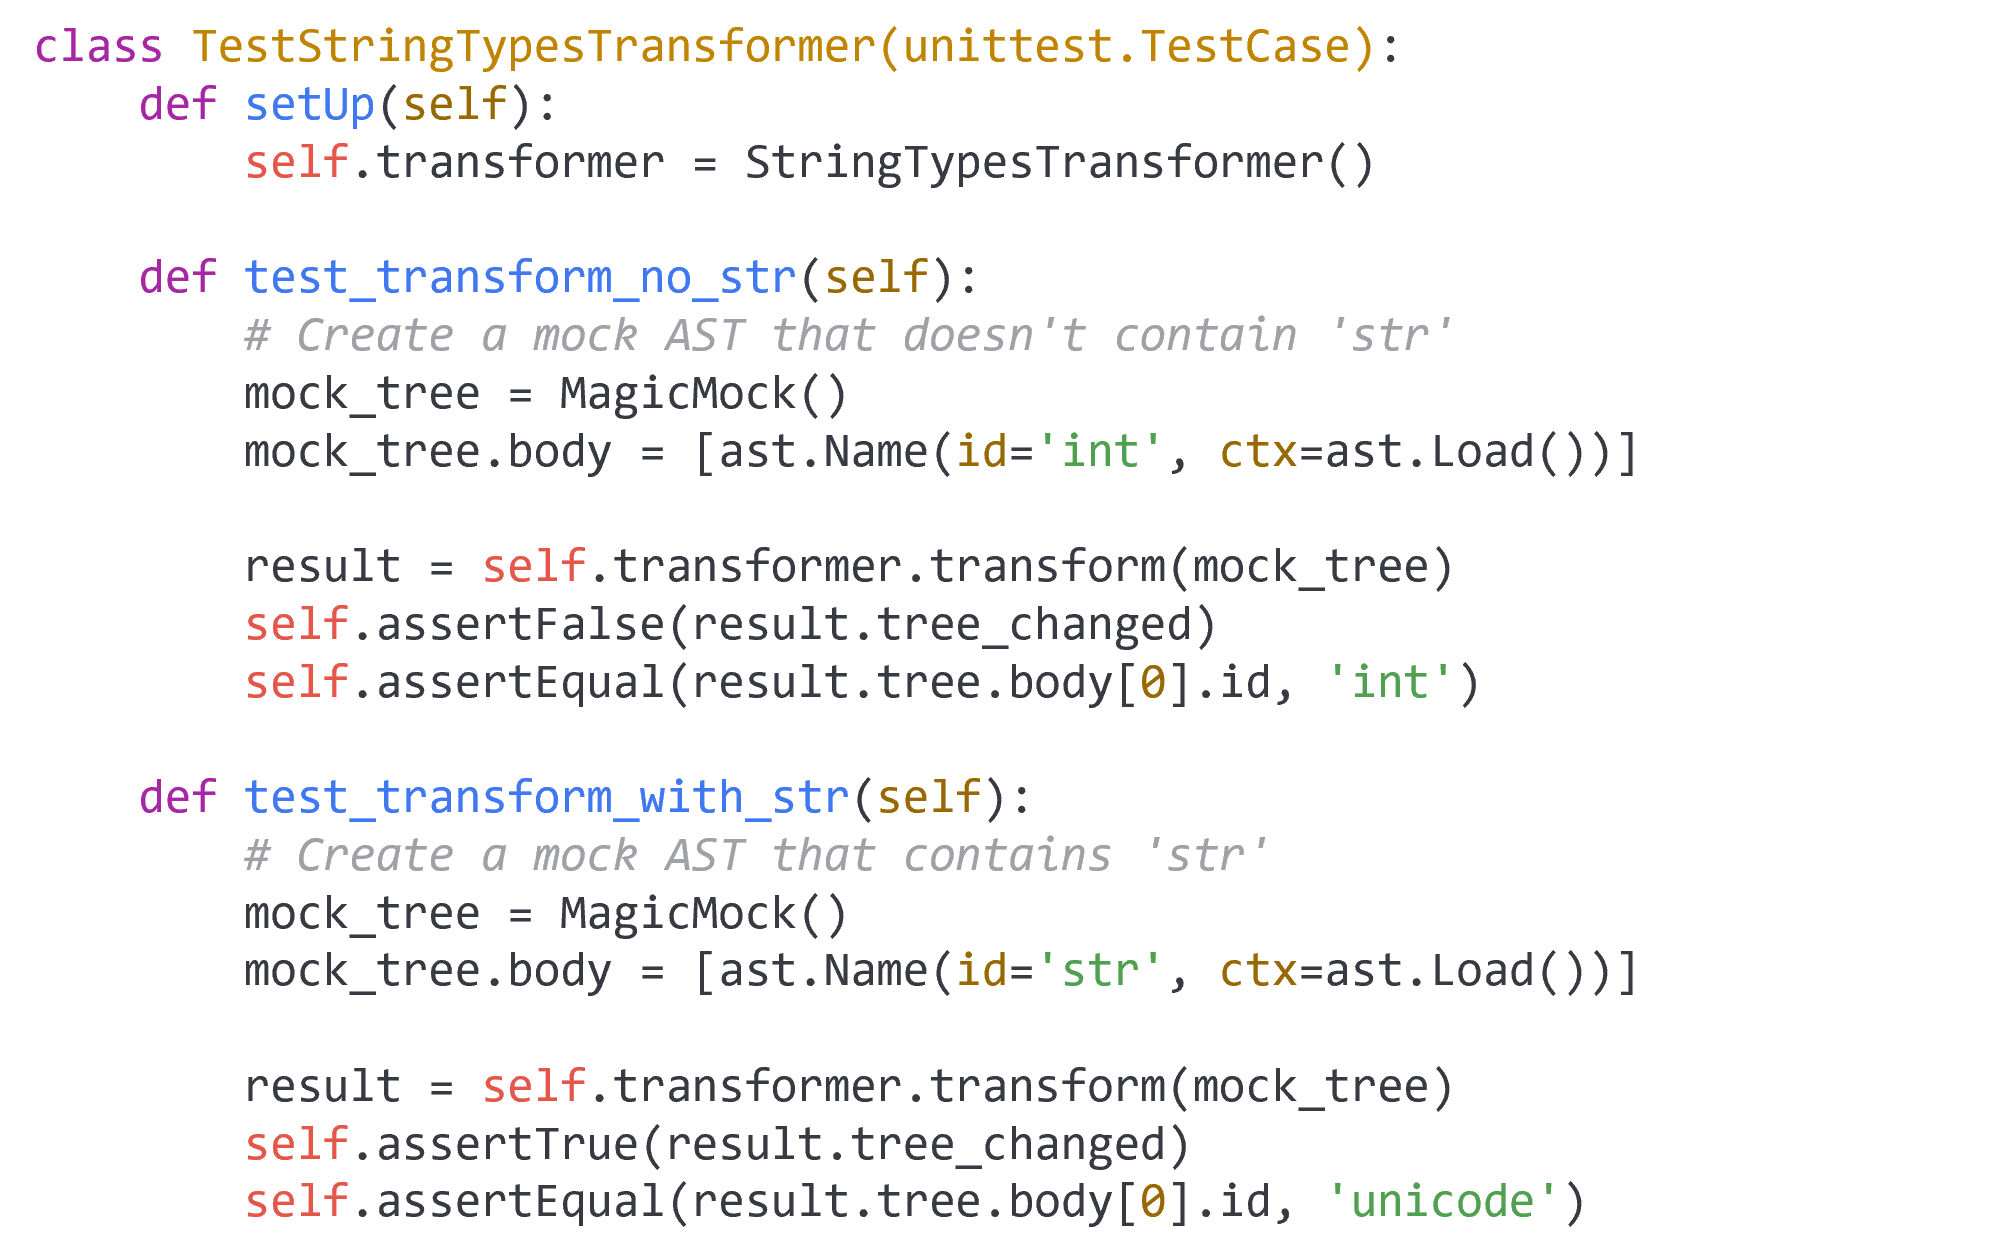}
        % \vspace{-10pt}
        \caption{Baseline GPT-4 generations.\label{fig:gpt_casestudy2:base}}
    \end{subfigure}
  \begin{subfigure}[b]{0.8\linewidth}
  \centering
        \includegraphics[width=\textwidth]{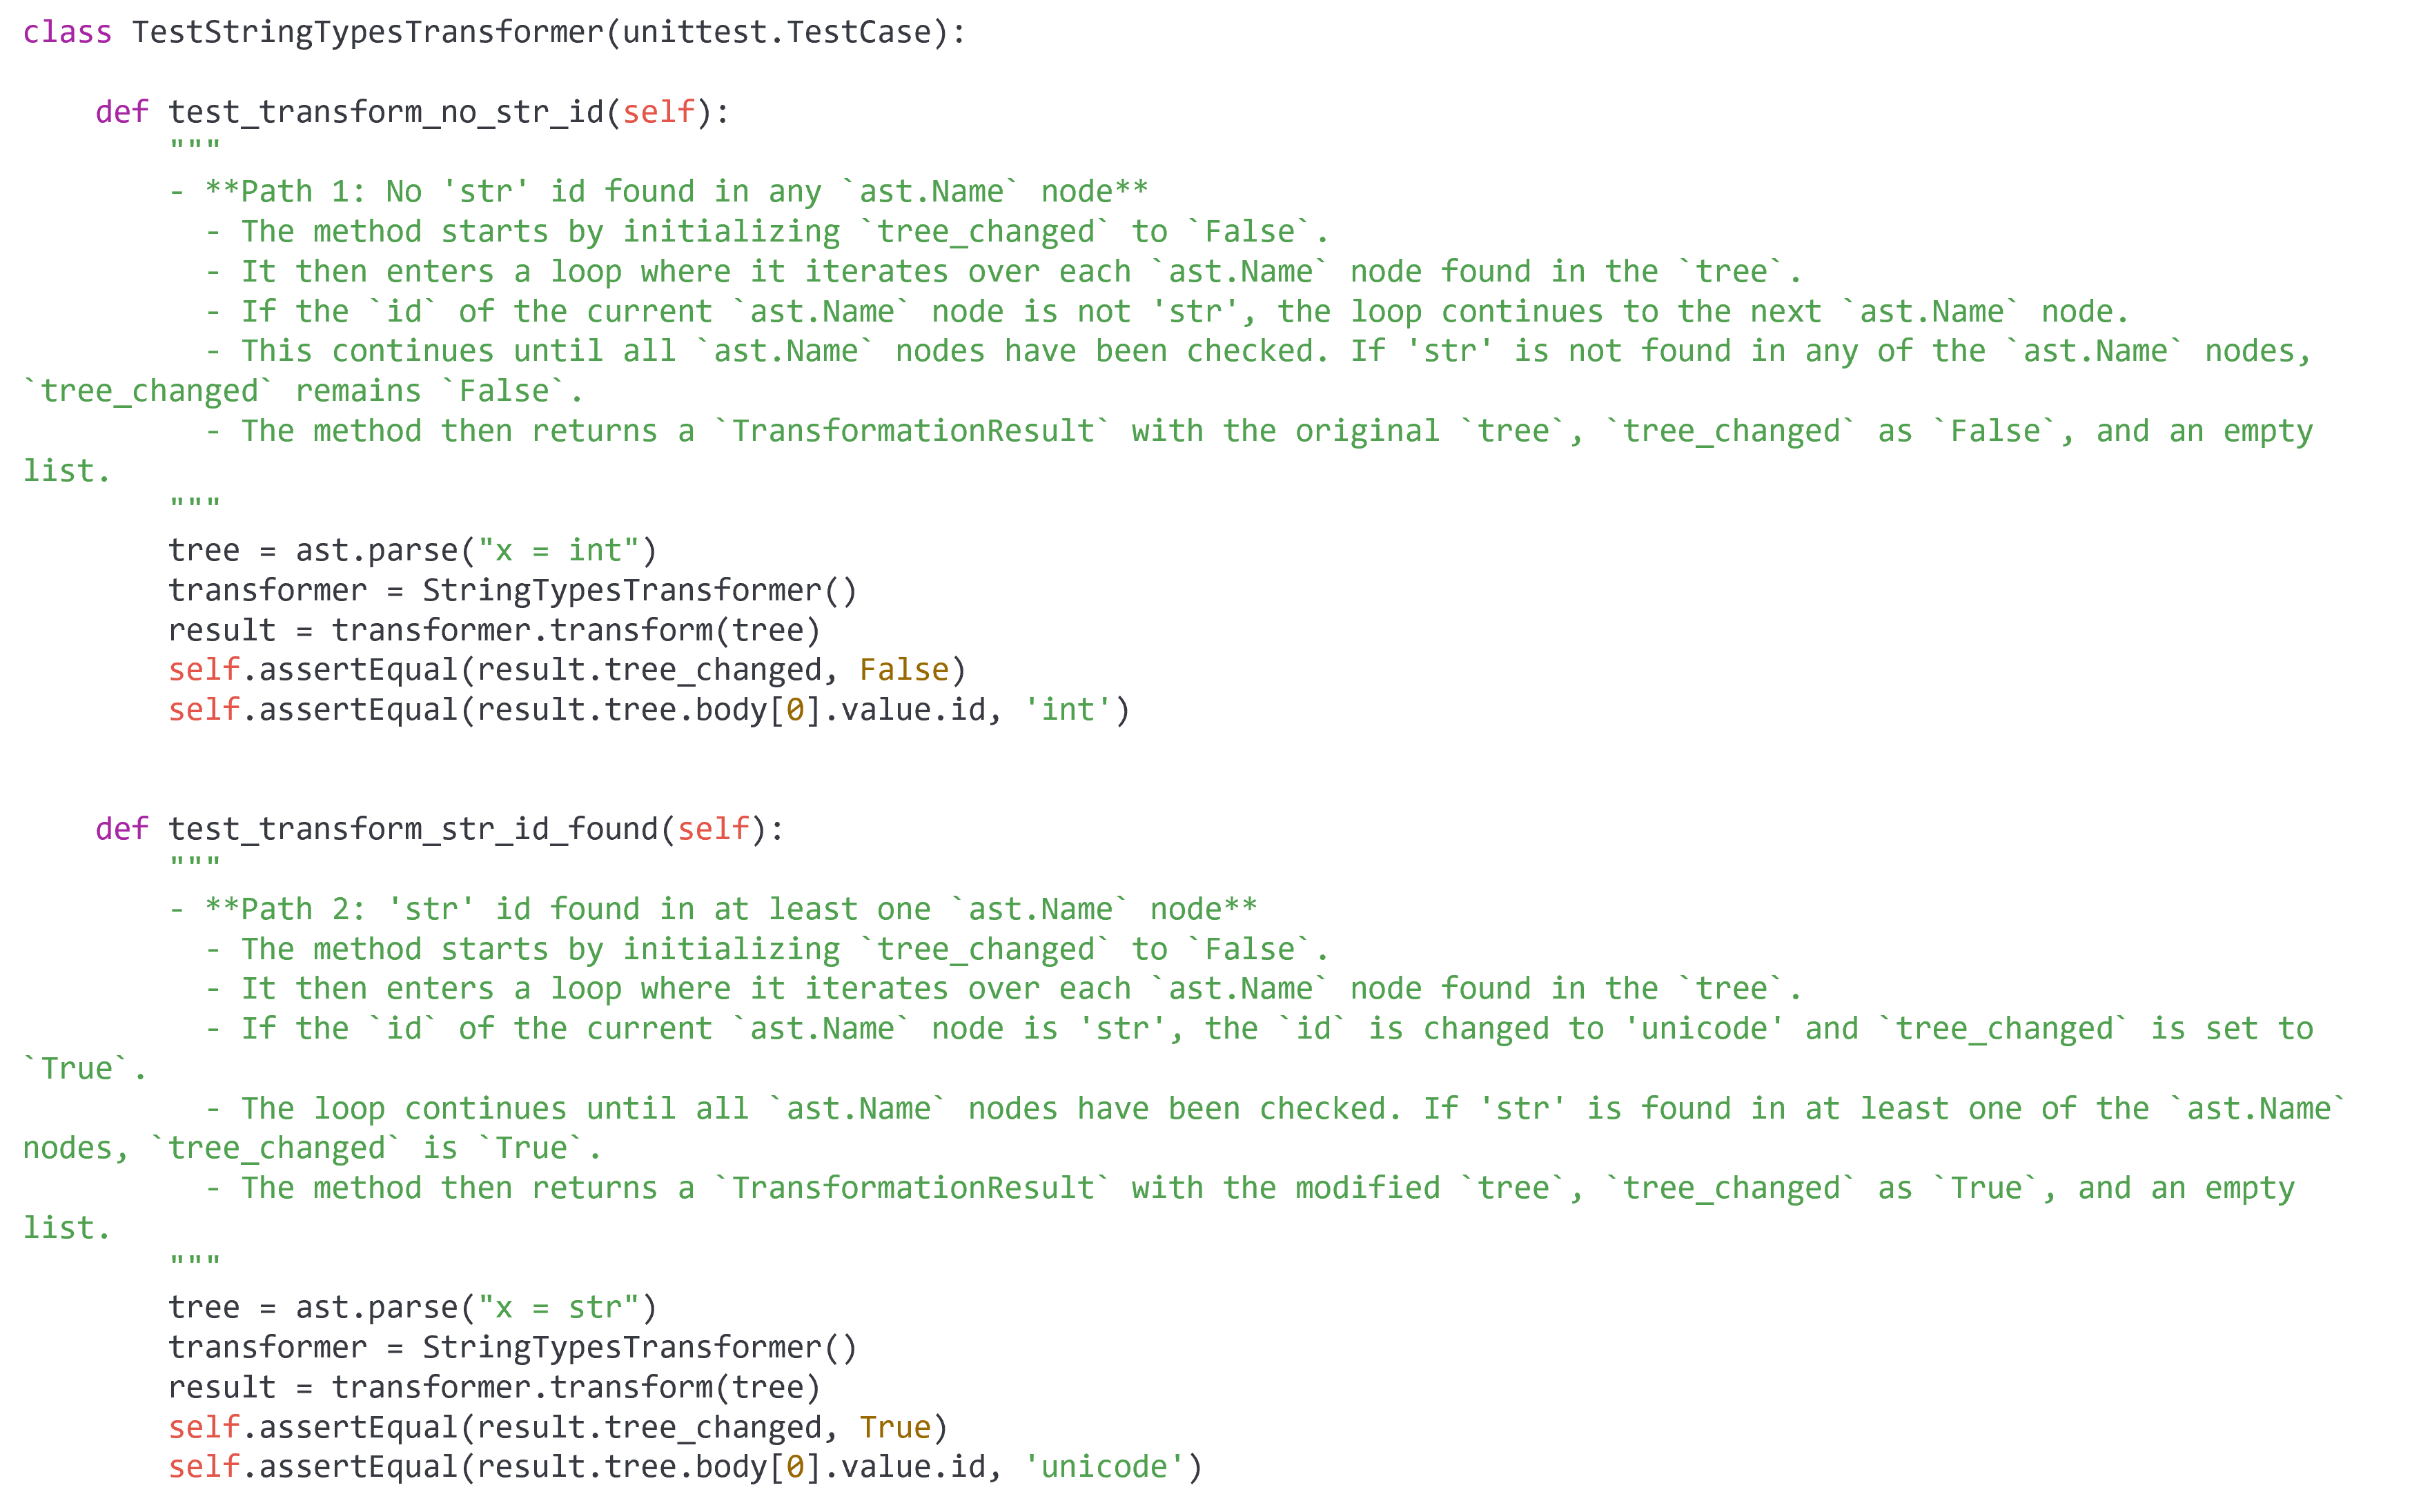}
        % \vspace{-10pt}
        \caption{GPT-4 generated tests.\label{fig:gpt_casestudy2:symgen}}
    \end{subfigure}
\caption{Case study showing GPT generations with path constraint prompts.\label{fig:baselines}}
\end{figure}
